# Supplementary material for: Interlayer coupling driven phase evolution in hyperbolic $1T$-TaS$_2$
Source: arXiv:2512.07508 source file (2025-12-08)
Supplement: Supplementary file 1 [file SM_TaS2.pdf]

# Supplemental Material: Interlayer coupling driven phase evolution in hyperbolic $1T$-TaS$_2$

Achyut Tiwari, Bruno Gompf, and Martin Dressel
*1. Physikalisches Institut, Universität Stuttgart, Pfaffenwaldring 57, 70569 Stuttgart, Germany*
(Dated: December 8, 2025)

## S1. SPECTROSCOPIC ELLIPSOMETRY AND FITTED PARAMETERS Ψ AND Δ AT T = 300 K

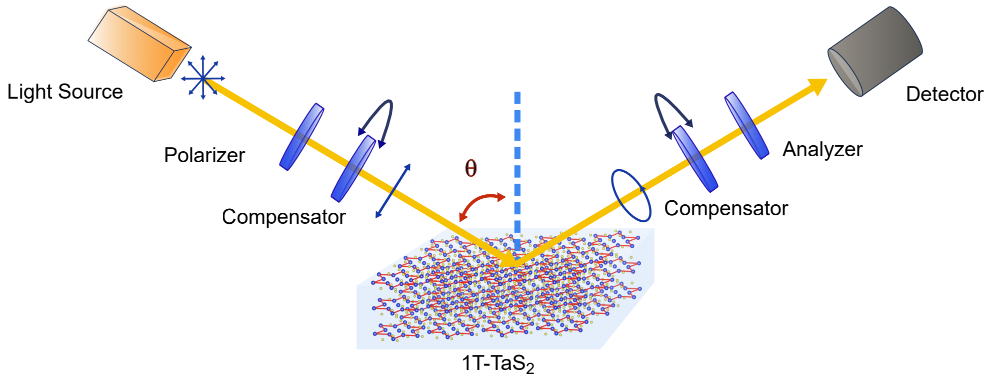


FIG. S1. Schematic of the ellipsometry measurement setup: Unpolarized light from the source passes through a polarizer and a rotating compensator before reflecting off the sample under multiple angles of incidence (AOIs), $\theta$. The reflected light then traverses a second rotating compensator and an analyzer before reaching the detector.

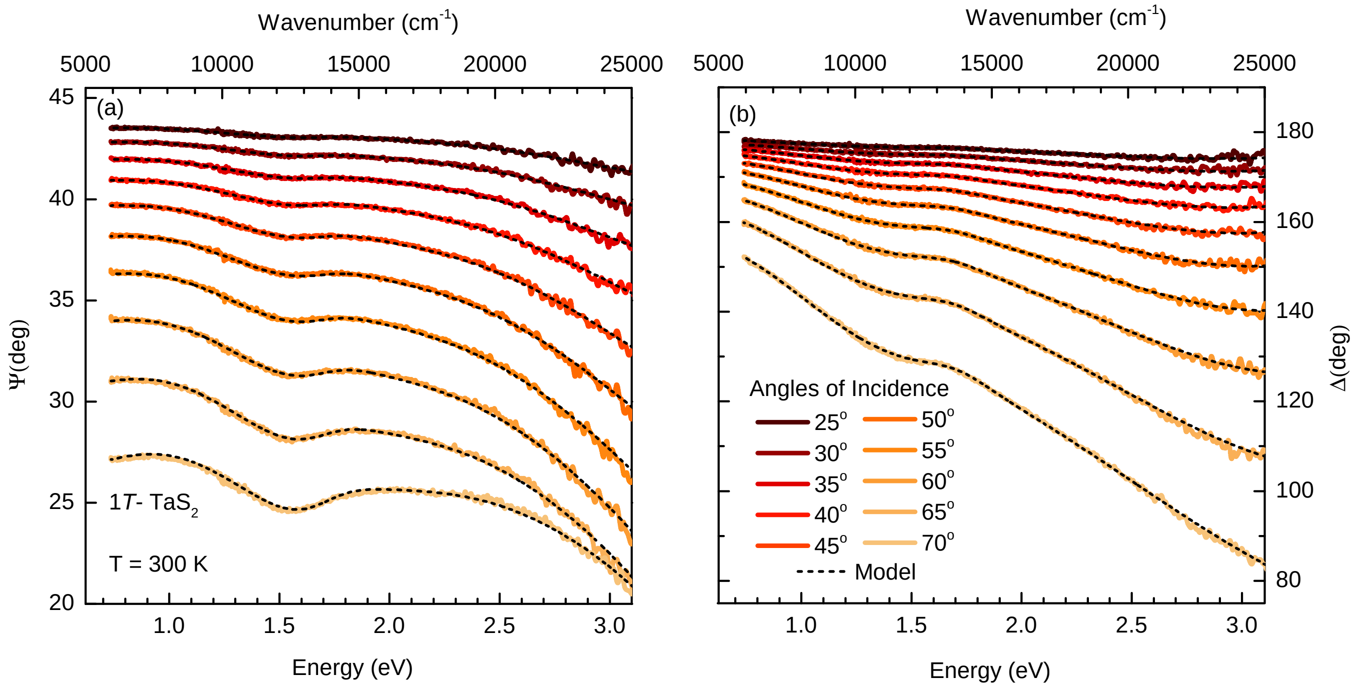


FIG. S2. Ellipsometric parameters Ψ and Δ for $1T$-TaS$_2$ *vs.* energy, for multiple angles of incidence at room temperature: experimental data (colored solid lines) and best match model (black dashed lines).

## S2. TEMPERATURE-DEPENDENT ELLIPSOMETRIC PARAMETERS Ψ AND Δ

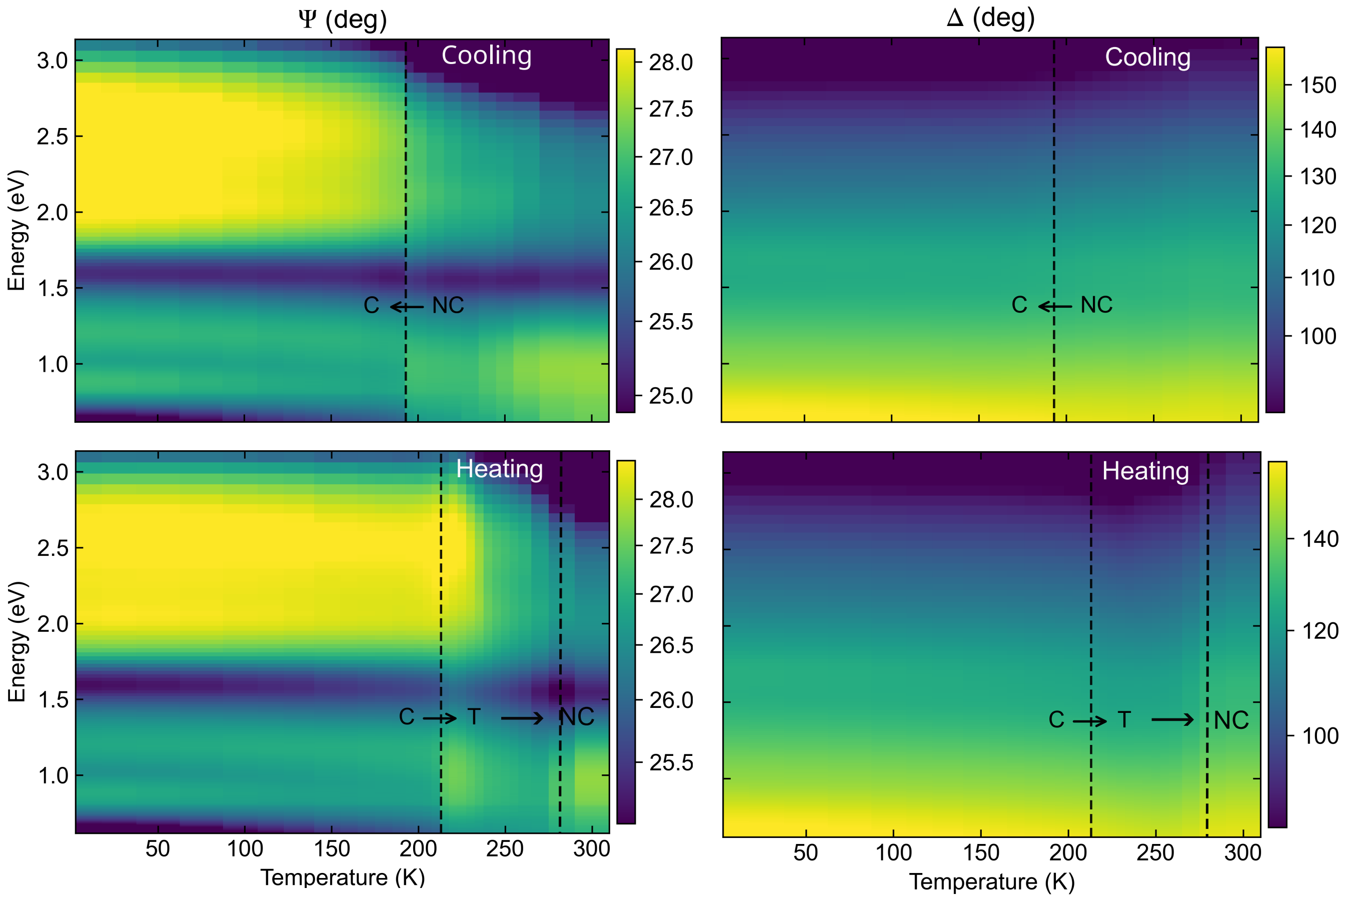


FIG. S3. Temperature-dependent ellipsometric parameters Ψ(T) and Δ(T) across the metal-insulator transition for cooling (upper panels) and heating (lower panels). Vertical dashed lines show the transition temperature from nearly commensurate (NC-metal) to commensurate (C-insulator) CDW upon cooling. Upon heating, it displays the hysteresis with an additional intemediate phase denoted as triclinic (T) phase.

## S3. THE EXPERIMENTAL AND CALCULATED ELLIPSOMETRIC PARAMETERS Ψ AND Δ FOR DIFFERENT TEMPERATURES ACROSS THE METAL-INSULATOR TRANSITION UPON COOLING

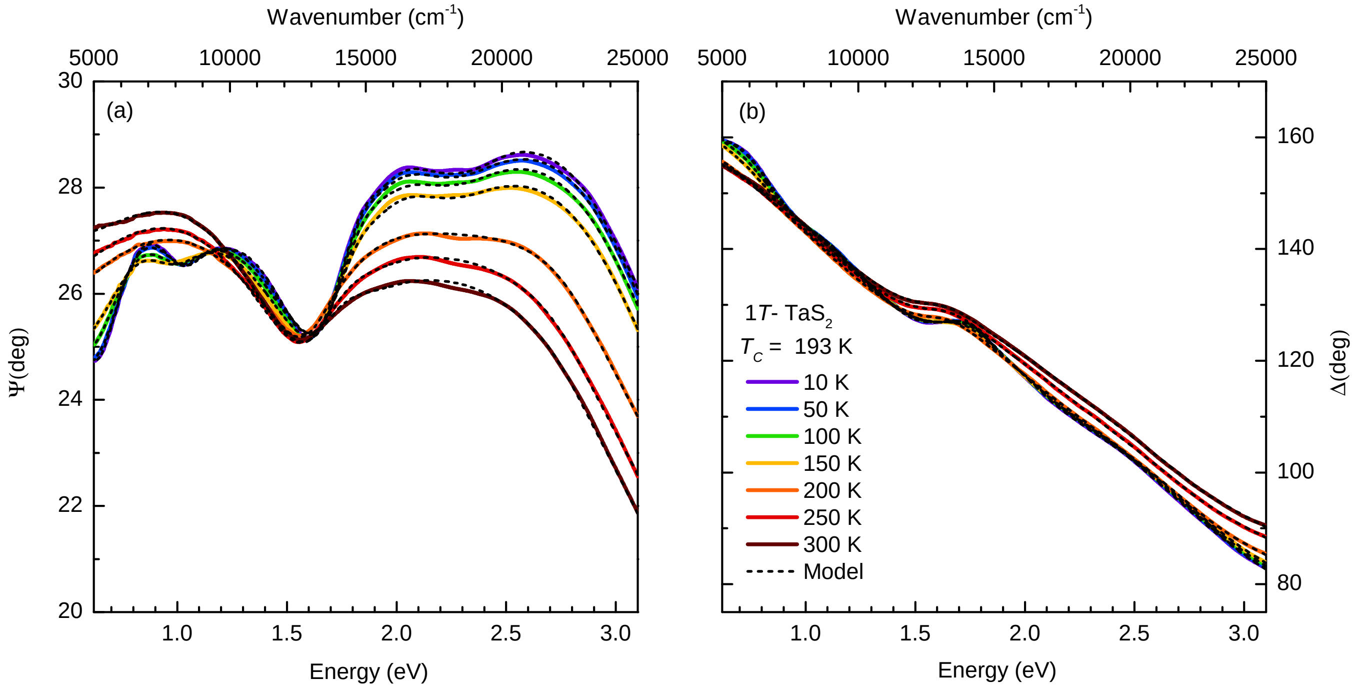


FIG. S4. Ellipsometric parameters Ψ and Δ for $1T$-$TaS_2$ *vs.* energy, at fixed AOI of $70^o$ for different temperatures across metal-insulator transition: experimental data (colored solid lines) and best match model (black dashed lines).

## S4. MODEL'S PARAMETERS OF USED OSCILLATORS TO FIT THE SPECTROSCOPIC ELLIPSOMETRY DATA

The complex dielectric function $\tilde{\varepsilon}(E)$ was modeled as a sum of Drude, Lorentz, and Tauc–Lorentz contributions, which account for the response of itinerant carriers and bound electronic excitations, respectively,

$$\tilde{\varepsilon}(E) = \varepsilon_{\mathrm{Drude}}(E) + \sum_n \varepsilon_{\mathrm{Lorentz},n}(E) + \sum_n \varepsilon_{\mathrm{TL},n}(E), \tag{S1}$$

where $E = \hbar\omega$ is the photon energy.

The Drude term describes the response of free (itinerant) carriers,

$$\varepsilon_{\mathrm{Drude}}(E) = \frac{-\hbar^2}{\varepsilon_0\,\rho_n\big(\tau_n E^2 + i\hbar E\big)}. \tag{S2}$$

Here, $\varepsilon_0$ is the vacuum permittivity, $\rho_n$ is the dc resistivity associated with the Drude channel $n$, and $\tau_n$ is the corresponding carrier relaxation time. This form is equivalent to the usual Drude expression in terms of plasma frequency and damping rate, but written in a way that uses $\rho_n$ and $\tau_n$ as fit parameters.

Interband transitions and other bound excitations are modeled with Lorentz oscillators,

$$\varepsilon_{\mathrm{Lorentz},n}(E) = \frac{A_n\,Br_n\,E_n}{E_n^2 - E^2 - i\,E\,Br_n}, \tag{S3}$$

where $A_n$ is the oscillator amplitude, $E_n$ is the resonance energy, and $Br_n$ is the broadening (damping) parameter for the $n$th Lorentz contribution. These terms account for discrete or relatively narrow-band transitions between occupied and unoccupied states.

Broad interband absorption onsets associated with a gap are described by Tauc–Lorentz (T-LO) oscillators. The complex T-LO contribution is written as

$$\varepsilon_{\mathrm{T-LO},n}(E) = \varepsilon_{1,n}(E) + i\,\varepsilon_{2,n}(E), \tag{S4}$$

with the imaginary part defined as

$$\varepsilon_{2,n}(E) = \begin{cases} \dfrac{A_n\,E_{0,n}\,Br_n\,(E-E_{\mathrm{g},n})^2}{E\left[(E^2-E_{0,n}^2)^2+Br_n^2E^2\right]} & \text{for } E > E_{\mathrm{g},n}, \\ 0 & \text{for } E \le E_{\mathrm{g},n}, \end{cases} \tag{S5}$$

and the real part obtained from the Kramers–Kronig relation,

$$\varepsilon_{1,n}(E) = \frac{2}{\pi}\,PV\int_{E_{\mathrm{g},n}}^{\infty} \frac{\omega\,\varepsilon_{2,n}(\omega)}{\omega^2-E^2}\,d\omega, \tag{S6}$$

where $PV$ denotes the Cauchy principal value of the integral.

Here, $A_n$ is the T-LO oscillator amplitude, $E_{0,n}$ is the T-LO resonance (central) energy, $Br_n$ is the broadening, and $E_{\mathrm{g},n}$ is the onset (Tauc) gap energy for the $n$th T-LO oscillator. The function $\varepsilon_{2,n}(E)$ vanishes below $E_{\mathrm{g},n}$, which enforces an optical gap, and rises smoothly above the onset, while $\varepsilon_{1,n}(E)$ is obtained by enforcing causality through the Kramers–Kronig transform as presented in Jellison and Modine [1, 2].

TABLE S1. **High temperature metallic phase at 300 K:** The parameters of the Drude, Tauc-Lorentz (T-LO) and Lorentz (LO) oscillators used to analyze the spectroscopic ellipsometric data at T = 300 K. The amplitude (A), center energy $E_n$ ($E_0$ in case of Tauc-Lorentz) and broadening of used oscillators has been determined by fitting the raw data. In the case of the Tauc-Lorentz oscillator, $E_g$ represents the band gap energy of corresponding transitions, and R represents the resistivity for the Drude component. The last digit with 90% confidence, which is indicated with parentheses for each parameter.

| T= 300 K | MSE: 1.74 | | | | | |
|---|---|---|---|---|---|---|
| | Oscillator | $A$ (eV) | $E_g$ (eV) | $E_0$ or $E_n$(eV) | Br (eV) | R (mΩ-cm) |
| In-plane | T-LO | 132.9(7) | 1.9(2) | 2.0(5) | 11.8(6) | - |
| | $LO_1$ | 25.7(2) | - | 0.9(1) | 1.3(7) | - |
| | $LO_2$ | 2.2(2) | - | 1.6(9) | 0.4(3) | - |
| | $LO_3$ | 6.1(6) | - | 2.1(0) | 1.4(1) | - |
| | Drude | - | - | - | - | 1.0(1) |
| Out-of-plane | T-LO | 78.5(3) | 1.4(3) | 1.4(7) | 6.7(0) | - |
| | $LO_1$ | 2.2(2) | - | 1.5(0) | 0.5(5) | - |
| | $LO_2$ | 1.5(3) | - | 2.7(7) | 0.8(1) | - |
| | Drude | - | - | - | - | 2.5(0) |

TABLE S2. **Low-temperature insulating phase at 100 K:** The parameters of the Tauc-Lorentz (T-LO) and Lorentz (LO) oscillators used to analyze the spectroscopic ellipsometric data at T = 100 K. The amplitude (A), center energy $E_n$ ($E_0$ in case of Tauc-Lorentz) and broadening of used oscillators has been determined by fitting the raw data. In the case of the Tauc-Lorentz oscillator, $E_g$ represents the band gap energy of corresponding transitions. The last digit with 90% confidence, which is indicated with parentheses for each parameter.

| T= 100 K | MSE: 2.18 | | | | |
|---|---|---|---|---|---|
| | Oscillator | $A$ (eV) | $E_g$ (eV) | $E_0$ or $E_n$(eV) | Br (eV) |
| In-plane | T-LO | 183.9(9) | 2.4(4) | 2.6(5) | 11.7(8) |
| | $LO_1$ | 16.0(9) | - | 1.2(6) | 1.3(4) |
| | $LO_2$ | 5.1(8) | - | 2.4(2) | 1.3(5) |
| | $LO_3$ | 6.9(5) | - | 1.7(9) | 0.4(5) |
| | $LO_4$ | 21.9(1) | - | 0.8(2) | 0.6(7) |
| | $LO_5$ | 5.97(6) | - | 0.5(9) | 0.2(5) |
| Out-of-plane | T-LO | 76.6(9) | 2.1(7) | 2.3(2) | 29.6(8) |
| | $LO_1$ | 5.5(3) | - | 1.7(4) | 0.5(6) |
| | $LO_2$ | 3.3(1) | - | 0.9(5) | 0.3(0) |
| | $LO_3$ | 4.9(2) | - | 2.7(6) | 0.9(8) |
| | $LO_4$ | 5.6(1) | - | 0.5(4) | 0.4(2) |

## S5. THE EXPERIMENTAL AND CALCULATED ELLIPSOMETRIC PARAMETERS Ψ AND Δ FOR DIFFERENT TEMPERATURES ACROSS MIT UPON HEATING

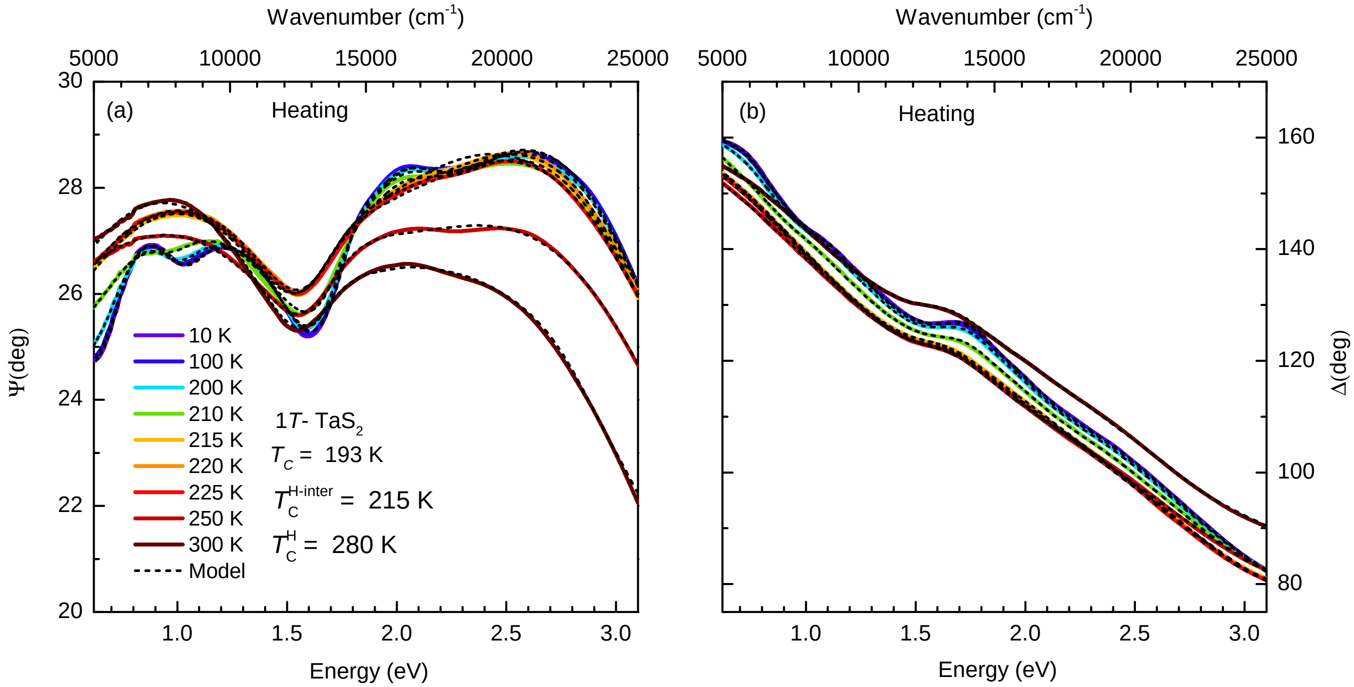


FIG. S5. Ellipsometric parameters Ψ and Δ as a function of energy for $1T$-$TaS_2$ at different temperatures across the metal–insulator transition during heating. Colored solid lines show the experimental data and black dashed lines show the best-fit model. For the 225 K heating, the same model used to fit the 300 K cooling data has been applied.

TABLE S3. **Intermediate phase at 225 K:** The parameters of the Drude, Tauc-Lorentz (T-LO) and Lorentz (LO) oscillators used to analyze the spectroscopic ellipsometric data at T = 225 K upon heating. The amplitude (A), center energy $E_n$ ($E_0$ in case of Tauc-Lorentz) and broadening of used oscillators has been determined by fitting the raw data. In the case of the Tauc-Lorentz oscillator, $E_g$ represents the band gap energy of corresponding transitions, and R represents the resistivity for the Drude component. The last digit with 90% confidence, which is indicated with parentheses for each parameter.

| T= 225 K (Heating) MSE: 1.4 | | | | | | |
|---|---|---|---|---|---|---|
| | Oscillator | $A$ (eV) | $E_g$ (eV) | $E_0$ or $E_n$(eV) | Br (eV) | R (mΩ-cm) |
| In-plane | T-LO | 77.9(5) | 1.9(0) | 2.0(5) | 11.8(5) | - |
| | $LO_1$ | 23.1(2) | - | 0.9(0) | 1.3(0) | - |
| | $LO_2$ | 2.2(2) | - | 1.6(9) | 0.5(1) | - |
| | $LO_3$ | 6.1(6) | - | 2.1(6) | 1.4(2) | - |
| | Drude | - | - | - | - | 1.7(9) |
| Out-of-plane | T-LO | 68.2(3) | 1.4(1) | 1.5(0) | 6.6(0) | - |
| | $LO_1$ | 2.9(7) | - | 1.5(0) | 0.5(4) | - |
| | $LO_2$ | 7.7(8) | - | 2.8(1) | 0.6(7) | - |
| | Drude | - | - | - | - | 1.9(6) |

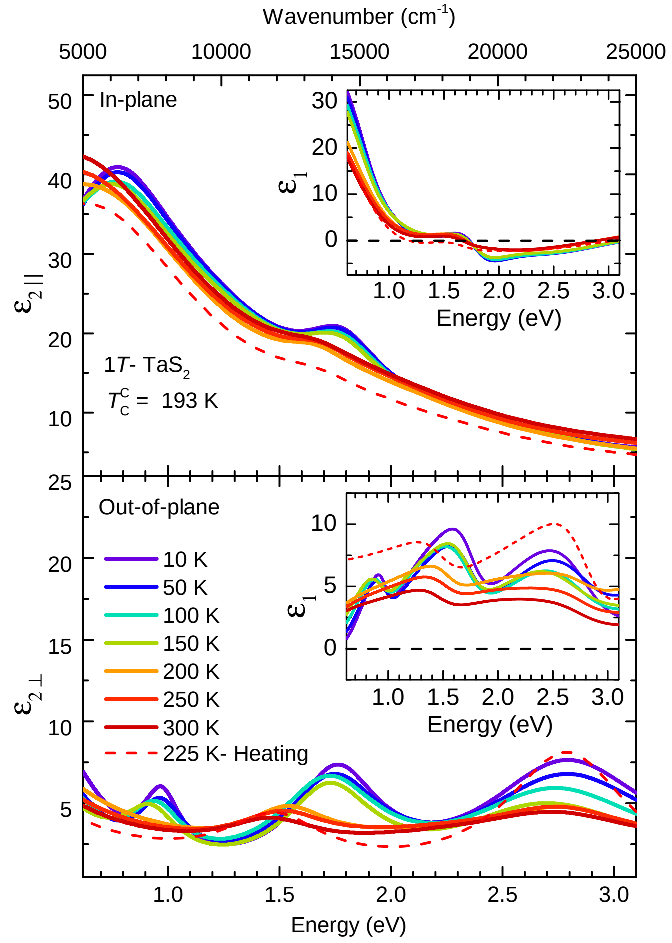


FIG. S6. **Dielectric function of intermediate phase at 225 K**, compared to Imaginary part of the complex dielectric function for in-plane (upper panel) and out-of-plane (lower panel) of 1$T$-$TaS_2$ *vs.* energy for different temperatures across MIT upon cooling. The inset shows the corresponding real part of complex dielectric function *vs.* energy for different temperatures across the metal-insulator transition. The distinct dielectric function at 225 K indicates that the phase transition takes separate microscopic pathways on the cooling and heating

## S6. THE EXPERIMENTAL ELLIPSOMETRIC PARAMETERS AND $a$BEMA MODEL FIT FOR DIFFERENT TEMPERATURES ACROSS THE METAL-INSULATOR TRANSITION

For the cooling, the dielectric function obtained (using oscillators as shown in section S4) for the low-temperature insulating phase (100 K) and high-temperature metallic phase (230 K) were kept fixed and only the metallic volume fraction and shape factor were allowed to vary in the $a$BEMA model. With these minimal parameters, the $a$BEMA model reproduces the spectra over a wide spectral range, with the deviations near the transition temperature.

For the heating, a two-component aBEMA description is not sufficient in the 225–280 K window. In this case, a three-component aBEMA model was used, based on the dielectric functions of the low-temperature insulating phase (100 K), the high-temperature metallic phase (300 K), and an intermediate phase around 225 K, all determined in the previous section. Only the phase volume fractions and a single shape factor were varied with temperature. This three-component aBEMA captures the main evolution of the ellipsometric spectra during heating.

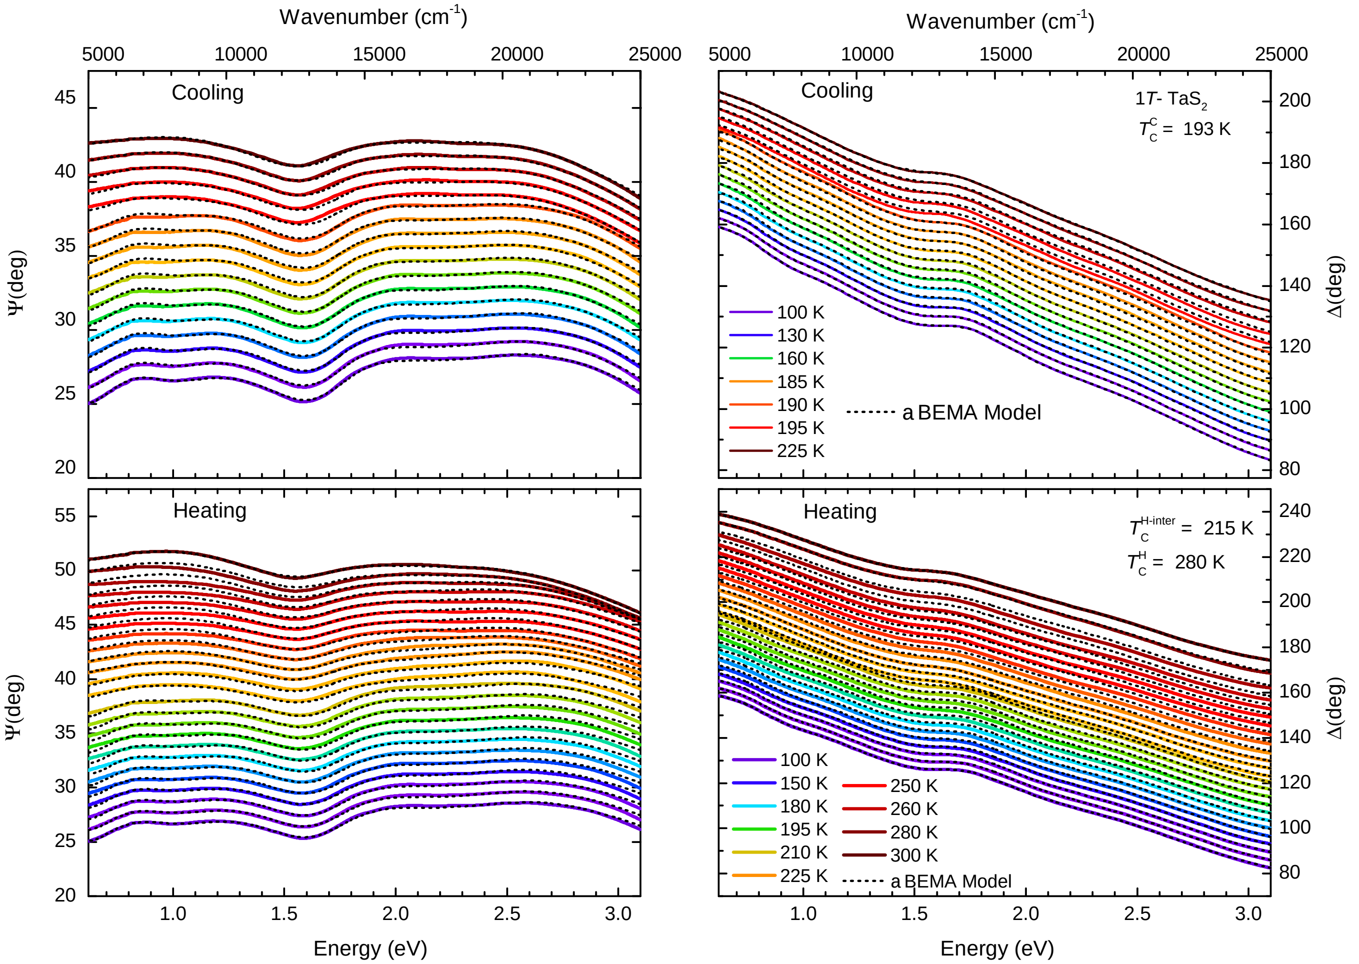


FIG. S7. Ellipsometric parameters Ψ and Δ as a function of energy for $1T$-$TaS_2$ in small temperature steps across the metal–insulator transition during cooling and heating. The colored solid curves show the experimental data, and black dashed curves show the best fits obtained from the $a$BEMA Model. For clarity, the spectra at different temperatures are vertically offset by a constant value.


[1] G. E. Jellison, Jr. and F. A. Modine, "Parameterization of the optical functions of amorphous materials in the interband region," Appl. Phys. Lett. **69**, 371–373 (1996).

[2] G. E. Jellison, Jr., "Erratum: 'Parameterization of the optical functions of amorphous materials in the interband region' [Appl. Phys. Lett. 69, 371 (1996)]," Appl. Phys. Lett. **69**, 2137 (1996).
